# Supplementary material for: Learning Scale-Free Networks by Dynamic Node-Specific Degree Prior
Source: arXiv:1503.02129 source file (2015-06-18)
Supplement: Supplementary file 3 [file Supp_Learning_Scale-Free_Networks_by_Dynamic_Node_Specific_Degree_Prior.pdf]

---

# Supplementary Material

---

February 6, 2015

In this draft, We try to prove theorem 1 and theorem 2.

## 1 PROOF OF THEOREM 1

**Theorem 1.** *The output ( $Y'$ ) of Algorithm 1 satisfying*

$$\arg \min \frac{1}{2} \|Y - A\|_F^2 + \lambda \sum_{v=1}^p g(v) Y_{[v, Y', h']} \circ H$$

*Proof.* Denote the output of Algorithm 1 is  $Y^{t+1}$ , which satisfies  $[Y^{t+1}, H, \delta^t] = [Y^t, H, \delta^t] = [Y^{t+1}, h']$ . So

$$\arg \min_Y \frac{1}{2} \|Y - A\|_F^2 + \lambda \sum_{i=1}^p g(v) Y_{[v, Y^{t+1}, h']} \circ H$$

is equivalent to

$$\arg \min_Y \frac{1}{2} \|Y - A\|_F^2 + \lambda \sum_{i=1}^p g(v) Y_{[v, Y^{t+1}, H, \delta^t]} \circ H$$

Since  $[Y^{t+1}, H, \delta^t] = [Y^t, H, \delta^t]$ , both  $\delta$  and the objective function would not change. Therefore  $Y^{t+1}$  is a solution to (18).  $\square$

## 2 PROOF OF THEOREM 2

Actually, the subprolem  $\left( (21) \text{ in the main paper} \right)$  can be written as

$$\frac{1}{2} \|Y_i - M_i\|_F^2 + \sum_{k=1}^{p-1} |Y_{i,(k)}| g(k) \tag{2.1}$$

Here,  $\{g(1), g(2), \dots, g(p-1)\}$  is a positive sequence. Given a feasible solution  $Y_i$ , obviously we can assume  $Y_{ii} = M_{ii}$ , otherwise  $Y_i$  can not be the optimal solution. In the following content, we do not consider the  $i^{th}$  component  $Y_{i,i}$  of  $Y_i$  and also the  $i^{th}$  component  $M_{i,i}$  of  $M_i$ . If we say rank the components of  $Y_i$  or  $M_i$ , we actually mean rank all the components excluding  $Y_{i,i}$  and  $M_{i,i}$ .

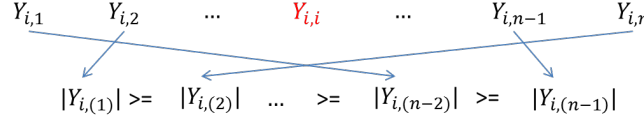

Figure 2.1: Rank solution. The one one correspondence is defined.

Sort all the components of  $Y_i$  based on the absolute value of each component, we get  $|Y_{i,(1)}| \geq |Y_{i,(2)}| \geq \dots \geq |Y_{i,(p-1)}|$  as shown in Figure 2.1. Obviously, there is one one correspondence between  $Y_{i,*}$  and  $Y_{i,(*)}$ . If  $Y_{i,j}$  corresponds to  $Y_{i,(k)}$ , then we denote the correspondence as  $Map(Y_{i,(k)}) = j$ .

Assume that  $|Y_{i,(1)}| = |Y_{i,(2)}| = \dots = |Y_{i,(t)}| > |Y_{i,(t+1)}|$ , we denote  $\{Y_{i,(1)}, Y_{i,(2)}, \dots, Y_{i,(t)}\}$  as  $C|_{Y_i}(1)$ . Similarly, we can construct  $C|_{Y_i}(2)$ ,  $C|_{Y_i}(3)$  and etc. Assume  $\cup_{k=1}^{n-1} Y_{i,(k)}$  can be clustered into  $T(Y_i)$  groups, that is  $\{C|_{Y_i}(1), C|_{Y_i}(2), \dots, C|_{Y_i}(T(Y_i))\}$ . We use  $|C|_{Y_i}(k)|$  to denote the number of elements in  $C|_{Y_i}(k)$ , and for each element of  $C|_{Y_i}(k)$ , the absolute value should equal to  $y|_{Y_i}(k)$ . When context is clear, we use  $C(k)$ ,  $\hat{C}(k)$ ,  $C'(k)$  and  $C^{(l)}(k)$  for  $Y_i$ ,  $\hat{Y}_i$ ,  $Y'_i$  and  $Y_i^{(l)}$  respectively. And we use  $y(k)$ ,  $\hat{y}(k)$ ,  $y'(k)$  and  $y^{(l)}(k)$  accordingly.

**Definition 1.** Given a feasible solution  $Y_i$ ,  $Y_i$  is a stable solution if and only if for each  $1 \leq j \leq T$ ,

$$y(j) = \max\left\{\frac{1}{|C(j)|} \sum_{s \in C(j)} [|M_{i, Map(Y_{i,(s)})}| - g(s)], 0\right\} \quad (2.2)$$

**Lemma 1.** The optimal solution  $Y_i^*$  is a stable solution.

**Proof.** First, we can rewrite the objective of (2.1) as follows,

$$\frac{1}{2} \sum_{j=1}^n (|Y_{i,j}| - |M_{i,j}|)^2 + \sum_{k=1}^{n-1} |Y_{i,(k)}| g(k) \quad (2.3)$$

Given a  $j$  such that  $1 \leq j \leq T$ , if  $y(j) \neq 0$ , we can calculate the gradient over the absolute value of elements in  $C(k)$ , and set it to 0, that is,

$$\sum_{s \in C(j)} \{|Y_{i,(s)}| - |M_{i, Map(Y_{i,(s)})}| + g(s)\} = 0 \quad (2.4)$$

Doing simple algebra yield the following equation,

$$y(j) = \frac{1}{|C(j)|} \sum_{s \in C(j)} [|M_{i, Map(Y_{i,(s)})}| - g(s)] \quad (2.5)$$

If  $y(k) = 0$ , we should calculate the sub-gradient, as follows,

$$\sum_{s \in C(j)} \{|Y_{i,(s)}| - |M_{i,Map(Y_{i,(s)})}| + \Gamma(|Y_{i,(s)}|)g(s)\} = 0 \quad (2.6)$$

From (2.6) it is easy to show that  $\sum_{s \in C(j)} [|M_{i,Map(Y_{i,(s)})}| - g(s)] \leq 0$  as  $0 \leq \Gamma(|Y_{i,(s)}|) \leq 1$ . Thus **Lemma 1** proved.

**Lemma 2.** *Solving (2.1) is equivalent to the following optimization problem,*

$$Max_{\hat{Y}_i} \sum_{k=1}^{n-1} \hat{Y}_{i,(k)}^2 \quad (2.7)$$

*subject to  $\hat{Y}_i$  is a stable solution.*

**Proof.** Given a stable solution  $\hat{Y}_i$ , the objective function of (2.1) can be re-written as the following form,

$$\frac{1}{2} \{ (Y_{i,i} - M_{i,i})^2 + [\sum_{j=1}^{\hat{T}} \sum_{s \in C(j)} (Y_{i,(s)} - \alpha_j)^2] + [\sum_{s=1}^{n-1} M_{i,(s)}^2] - [\sum_{j=1}^{\hat{T}} |\hat{C}(j)| \alpha_j^2] \} \quad (2.8)$$

where  $\alpha_*$  is the number after completing the square terms. It is easy to show that  $\alpha_j = \hat{y}(j)$  for  $1 \leq j \leq \hat{T}$ . Otherwise,  $\hat{Y}_i$  would not be a stable solution as  $\hat{Y}_i$  can not make gradients in different directions to 0. Lead to a contradiction. Substitute  $\hat{Y}_i$  to (2.8), we have

$$\frac{1}{2} [\sum_{s=1}^{n-1} M_{i,(s)}^2 - \sum_{j=1}^{\hat{T}} |\hat{C}(j)| \hat{y}(j)^2] \quad (2.9)$$

So it is reasonable to conclude that solving (2.1) is equivalent to maximize  $\sum_{j=1}^{\hat{T}} |\hat{C}(j)| \hat{y}(j)^2$  in the space of all stable solutions. Obviously, we have

$$\sum_{j=1}^{\hat{T}} |\hat{C}(j)| \hat{y}(j)^2 = \sum_{k=1}^{n-1} \hat{Y}_{i,(k)}^2 \quad (2.10)$$

Thus we conclude that **Lemma 2** is correct. Based on **Lemma 2**, we can define the partial relationship among stable solutions.

**Definition 2.** *Given two stable solutions  $Y_i^{(1)}$  and  $Y_i^{(2)}$ , we say  $Y_i^{(1)} > Y_i^{(2)}$  if and only if the following inequality holds*

$$\sum_{j=1}^{n-1} Y_{i,(j)}^{(1)2} > \sum_{j=1}^{n-1} Y_{i,(j)}^{(2)2} \quad (2.11)$$

Obviously, given the optimal solution  $Y_i^*$ , there is no such a feasible solution  $Y_i$  such that  $Y_i > Y_i^*$ . Based upon **Lemma 1**, we propose the following **Lemma 3**.

**Theorem 2.** Sort all components of  $M_i$  based on their absolute values, such that  $|M_{i,(1)}| \geq |M_{i,(2)}| \geq \dots \geq |M_{i,(n-1)}|$ . Given the optimal solution  $Y_i^*$ , for every  $j$  such that  $1 \leq j \leq T^*$ , we have

$$y^*(j) = \max\left\{\frac{1}{|C^*(j)|} \sum_{s \in C(j)} [|M_{i,(s)}| - g(s)], 0\right\} \quad (2.12)$$

Before proving **Theorem 2**, we show the following lemma.

**Lemma 3.** Given a non-negative non-decreasing sequence  $\{x_1, x_2, \dots, x_n\}$ . Given a set of non-negative numbers  $\{\delta_1, \delta_2, \dots, \delta_n\}$  satisfying  $\sum_{i=1}^s \delta_i \geq \sum_{i=s+1}^n \delta_i > 0$ . Then we have the following inequality holds,

$$\sum_{i=1}^s (x_i + \delta_i)^2 + \sum_{i=s+1}^n (x_i - \delta_i)^2 \geq \sum_{i=1}^n x_i^2 \quad (2.13)$$

**Proof.**

$$\begin{aligned} \sum_{i=1}^s (x_i + \delta_i)^2 + \sum_{i=s+1}^n (x_i - \delta_i)^2 &= \sum_{i=1}^n x_i^2 + \sum_{i=1}^n \delta_i^2 + 2\left[\sum_{i=1}^s x_i \delta_i - \sum_{i=s+1}^n x_i \delta_i\right] \\ &\geq \sum_{i=1}^n x_i^2 + \sum_{i=1}^n \delta_i^2 + 2\left[\sum_{i=1}^s x_s \delta_i - \sum_{i=s+1}^n x_{s+1} \delta_i\right] \\ &= \sum_{i=1}^n x_i^2 + \sum_{i=1}^n \delta_i^2 + 2\left[x_s \sum_{i=1}^s \delta_i - x_{s+1} \sum_{i=s+1}^n \delta_i\right] \\ &\geq \sum_{i=1}^n x_i^2 + \sum_{i=1}^n \delta_i^2 + [(x_s - x_{s+1})] \sum_{i=1}^n \delta_i \\ &\geq \sum_{i=1}^n x_i^2 + \sum_{i=1}^n \delta_i^2 \\ &\geq \sum_{i=1}^n x_i^2 \end{aligned}$$

Note that strict inequality always holds for (2.13) if  $\{x_1, x_2, \dots, x_n\}$  is not a constant sequence. Prove **Theorem 2** is equivalent to prove the following **Lemma 4**.

**Lemma 4.** Given the optimal solution  $Y_i^*$ , for every  $j$  such that  $1 \leq j \leq T^*$ , the following two sets are equal,

$$\begin{aligned} &\{M_{i, \text{Map}(Y_{i, (\sum_{x=1}^{j-1} |C^*(x)|+1)})}, M_{i, \text{Map}(Y_{i, (\sum_{x=1}^{j-1} |C^*(x)|+2)}), \dots, M_{i, \text{Map}(Y_{i, (\sum_{x=1}^j |C^*(x)|)}})\} \\ &\{M_{i, (\sum_{x=1}^{j-1} |C^*(x)|+1)}, M_{i, (\sum_{x=1}^{j-1} |C^*(x)|+2)}, \dots, M_{i, (\sum_{x=1}^j |C^*(x)|)}\} \end{aligned}$$

Actually, to prove **Lemma 4**, we just need to prove the following lemma, which is much easier to prove.

**Lemma 5.** Given a stable solution  $Y_i^{(0)}$ . If there exists a number  $p^{(0)}$  ( $1 \leq j \leq T^{(0)}$ ) and two numbers  $s_1, s_2$  where  $\sum_{x=1}^{p^{(0)}-1} |C(x)| < s_1 \leq \sum_{x=1}^{p^{(0)}} |C(x)|$  and  $\sum_{x=1}^{p^{(0)}} |C(x)| < s_2 \leq \sum_{x=1}^{p^{(0)}+1} |C(x)|$ , such that  $M_{i, \text{Map}^{(0)}(Y_{i,(s_1)})} < M_{i, \text{Map}^{(0)}(Y_{i,(s_2)})}$ , then there is another stable solution  $Y_i'$ , such that  $Y_i' > Y_i$ .

**Proof.** To prove **Lemma 5**, we just need to show that we can construct such kind a  $Y_i'$  described in **Lemma 5**.

We first construct  $Y_i^{(1)}$ . We set  $\text{Map}^{(1)}(Y_{i,(s_1)}) = \text{Map}^{(0)}(Y_{i,(s_2)})$  and  $\text{Map}^{(1)}(Y_{i,(s_2)}) = \text{Map}^{(0)}(Y_{i,(s_1)})$ . Then set each component of  $Y_i^{(1)}$  as follows,

$$\begin{aligned} Y_{i,i}^{(1)} &= Y_{i,i}^{(0)} \\ Y_{i,(s)}^{(1)} &= Y_{i,(s)}^{(0)} \quad \text{if} \quad 1 \leq s \leq \sum_{x=1}^{p^{(0)}-1} |C^{(0)}(x)| \quad \text{or} \quad \sum_{x=1}^{p^{(0)}+1} |C^{(0)}(x)| < s \leq n-1 \\ Y_{i,(s)}^{(1)} &= \frac{1}{|C^{(0)}(p^{(0)})|} \sum_{j \in C(p^{(0)})} [|M_{i, \text{Map}^{(1)}(Y_{i,(j)})} - g(j)] \quad \text{if} \quad \sum_{x=1}^{p^{(0)}-1} |C(x)| < s \leq \sum_{x=1}^{p^{(0)}} |C(x)| \\ Y_{i,(s)}^{(1)} &= \frac{1}{|C^{(0)}(p^{(0)}+1)|} \sum_{j \in C(p^{(0)}+1)} [|M_{i, \text{Map}^{(1)}(Y_{i,(j)})} - g(j)] \quad \text{if} \quad \sum_{x=1}^{p^{(0)}} |C(x)| < s \leq \sum_{x=1}^{p^{(0)}+1} |C(x)| \end{aligned}$$

By this way,  $Y_i^{(1)}$  is obviously "stable". If  $Y_i^{(1)}$  is also consistent, say satisfying the following condition, we say that  $Y_i^{(1)}$  is already a stable solution, and we denote  $Y_i' = Y_i^{(1)}$ .

$$y^{(1)}(p^{(1)} - 1) > y^{(1)}(p^{(1)}) > y^{(1)}(p^{(1)} + 1) > y^{(1)}(p^{(1)} + 2) \quad (2.14)$$

Otherwise, denote  $p^{(1)} = p^{(0)}$  and  $l^{(1)} = p^{(0)} + 1$ , and continue the following process. Assume that we have constructed  $Y_i^{(k)}$ . We say that  $Y_i^{(k)}$  is "left-consistent" if

$$y^{(k)}(p^{(k)}) < y^{(k)}(p^{(k)} - 1) \quad (2.15)$$

And similarly, we say that  $Y_i^{(k)}$  is "right-consistent" if,

$$y^{(k)}(p^{(k)} + 2) < y^{(k)}(p^{(k)} + 1) \quad (2.16)$$

Then we start to construct  $Y_i^{(k+1)}$ . If  $Y_i^{(k)}$  is not "left-consistent", set  $p^{(k+1)} = p^{(k)} - 1$ , merge  $C^{(k)}(p^{(k)})$  and  $C^{(k)}(p^{(k)} - 1)$  to one group  $C^{(k+1)}(p^{(k+1)})$  and set  $y^{(k+1)}(p^{(k+1)})$  as follows,

$$y^{(k+1)}(p^{(k+1)}) = \frac{|C^{(k)}(p^{(k)} - 1)|y^{(k)}(p^{(k)} - 1) + |C^{(k)}(p^{(k)})|y^{(k)}(p^{(k)})}{|C^{(k)}(p^{(k)} - 1)| + |C^{(k)}(p^{(k)})|} \quad (2.17)$$

Otherwise, set  $p^{(k+1)} = p^{(k)}$ , and set  $y^{(k+1)}(p^{(k+1)}) = y^{(k)}(p^{(k)})$ .

Also, if  $Y_i^{(k)}$  is not "right-consistent", then merge  $C^{(k)}(p^{(k)} + 1)$  and  $C^{(k)}(p^{(k)} + 2)$  into one group  $C^{(k+1)}(p^{(k+1)} + 1)$ . Set  $l^{(k+1)} = l^{(k)} + 1$ , and set  $y^{(k+1)}(p^{(k+1)} + 1)$  as follows,

$$y^{(k+1)}(p^{(k+1)} + 1) = \frac{|C^{(k)}(p^{(k)} + 1)|y^{(k)}(p^{(k)} + 1) + |C^{(k)}(p^{(k)} + 2)|y^{(k)}(p^{(k)} + 2)}{|C^{(k)}(p^{(k)} + 1)| + |C^{(k)}(p^{(k)} + 2)|} \quad (2.18)$$

Otherwise, set  $l^{(k+1)} = l^{(k+1)}$  and  $y^{(k+1)}(p^{(k+1)} + 1) = y^{(k)}(p^{(k)} + 1)$ . We then construct the rest part of  $Y_i^{(k+1)}$  as follows,

$$\begin{aligned} Y_{i,i}^{(k+1)} &= Y_{i,i}^{(k)} \\ Y_{i,(s)}^{(k+1)} &= Y_{i,(s)}^{(k)} \quad \text{if } 1 \leq s \leq \sum_{x=1}^{p^{(k+1)}-1} |C^{(k)}(x)| \\ Y_{i,(s)}^{(k+1)} &= Y_{i,(s)}^{(k)} \quad \text{if } \sum_{x=1}^{p^{(k+1)}} |C^{(k+1)}(x)| < s < n \end{aligned}$$

Then we get a new solution  $Y_i^{(k+1)}$ . It is easy to prove that  $Y_i^{(k+1)}$  is stable, if  $Y_i^{(k+1)}$  is also consistent, then we denote  $Y'_i = Y_i^{(k+1)}$ . Otherwise, we continue the process above to construct  $Y_i^{(k+2)}$ . Note that we would definitely stop as such kind of construction process will not go on forever.

When the process stopped, we would definitely get a stable solution  $Y'_i$ . We now prove that  $Y'_i > Y_i$  by showing the following inequality holds,

$$\sum_{a=p'}^{l'} |C^{(0)}(a)| y^{(0)}(a)^2 < |C'(p')| y'(p')^2 + |C'(p'+1)| y'(p'+1)^2 \quad (2.19)$$

If  $y'(p'+1) \neq 0$ , we have the following equality holds,

$$\sum_{a=p'}^{p^{(1)}} Y'_{i,a} - Y_{i,a} = \sum_{a=l^{(1)}}^{l'} Y_{i,a} - Y'_{i,a} \quad (2.20)$$

If  $y'(p'+1) = 0$ , then we have

$$\sum_{a=p'}^{p^{(1)}} Y'_{i,a} - Y_{i,a} > \sum_{a=l^{(1)}}^{l'} Y_{i,a} - Y'_{i,a} \quad (2.21)$$

According to **Lemma 3** we have

$$\sum_{a=p'}^{l'} |C^{(0)}(a)| y^{(0)}(a)^2 = \sum_{a=p'}^{l'} Y_{i,a}^2 < \sum_{a=p'}^{l'} Y'_{i,a}^2 = |C'(p')| y'(p')^2 + |C'(p'+1)| y'(p'+1)^2 \quad (2.22)$$

**Lemma 4, Lemma 5 and Theorem 2** proved.

Based on **Theorem 2**, solving (2.1) can be reduced to partitioning an ordered sequence into optimal blocks, as shown in Figure 3.1.

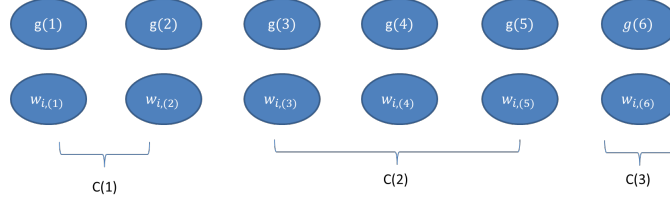

Figure 3.1: Partition Ordered Sequence

### 3 PROOF OF SUBSTRUCTURE PROPERTY

We use  $E(b)$  to denote the optimal partition over  $\{1, 2, \dots, b\}$ . And use  $B(a, b)$  to denote a block  $\{a, a+1, \dots, b\}$ . Then we have the following recursive function

$$E(b) = \min_{1 \leq x \leq b} B(x, b) \cup E(x-1) \text{ is consistent} \{B(x, b) \cup E(x-1)\} \quad (3.1)$$

We can design a  $O(n^2)$  dynamic programming algorithm to solve such an optimal partitioning problem. Can we do even faster? Actually, we have the following **Theorem 3**.

**Theorem 3.** Given stable solutions  $Y_i$  and  $Y'_i$ ,  $Y'_i > Y_i$  if and only if there is a number  $q$  where  $1 \leq q \leq \min(T, T')$ , such that

$$\begin{aligned} \text{for } 1 \leq s < q, \quad y(s) &= y'(s) \\ \text{for } q \quad y(q) < y'(q) \text{ or } y(q) &= y'(q) \text{ and } |c(q)| < |c'(q)| \end{aligned}$$

**Proof.** We prove **Theorem 3** by prove the following two conclusions.

- Given a stable solution  $Y_i$  and a number  $p$  where  $1 \leq p < T$  and a number  $s$  where  $\sum_{x=1}^p |C(x)| < s \leq \sum_{x=1}^{p+1} |C(x)|$ . If  $y(p) < \frac{y(p)|C(p)| + \sum_{s'=\sum_{x=1}^p |C(x)|+1}^s |W_{i(s')}| - g(s')}{|C(p)| + s - \sum_{x=1}^p |C(x)|}$ , there exists a stable solution  $Y'_i$ , such that  $Y'_i > Y_i$ .
- Given a stable solution  $Y_i$  and a number  $p$  where  $1 \leq p < T$  and a number  $s$  where  $\sum_{x=1}^{p-1} |C(x)| < s \leq \sum_{x=1}^p |C(x)|$ . If  $y(p) < \frac{\sum_{s'=\sum_{x=1}^{p-1} |C(x)|+1}^s |W_{i(s')}| - g(s')}{s - \sum_{x=1}^p |C(x)|}$ , there exists a stable solution  $Y'_i$ , such that  $Y'_i > Y_i$ .

We can prove the two conclusions by constructing corresponding  $Y'_i$ . The process to construct the  $Y'_i$  is similar to the process in the proof of **Lemma 5**, so we skip this part.

Based on **Theorem 3**, we can reduce the searching space of (3.1), as follows,

$$E(b) = \min_{1 \leq j \leq T_{b-1}} \left\{ \bigcup_{x=1}^{j-1} C_{b-1}(x) \cup B\left(\sum_{x=1}^{j-1} |C_{b-1}(x)| + 1, b\right) \right\} \quad (3.2)$$

Note that the optimization of (3.1) should be constrained in consistent solution space, that is, only consistent  $\bigcup_{x=1}^{j-1} C_{b-1}(x) \cup B(\sum_{x=1}^{j-1} |C_{b-1}(x)| + 1, b)$  is considered. Here,  $C_{b-1}(\ast)$  are the

groups of  $E(b-1)$  (refer to the definition of stable solution and their groups),  $T_{b-1}$  is the number of groups of  $E(b-1)$ . (3.2) shows that calculate  $E(b)$  only relies on  $E(b-1)$ . Actually, based on **Theorem 3**, it is easy to show the following two properties hold,

- If  $\bigcup_{x=1}^{j-1} C_{b-1}(x) \cup B(\sum_{x=1}^{j-1} |C_{b-1}(x)| + 1, b)$  is not consistent, then  $\bigcup_{x=1}^{j-2} C_{b-1}(x) \cup B(\sum_{x=1}^{j-2} |C_{b-1}(x)| + 1, b)$  is also not consistent.
- If both  $\bigcup_{x=1}^{j-1} C_{b-1}(x) \cup B(\sum_{x=1}^{j-1} |C_{b-1}(x)| + 1, b)$  and  $\bigcup_{x=1}^{j-2} C_{b-1}(x) \cup B(\sum_{x=1}^{j-2} |C_{b-1}(x)| + 1, b)$  are consistent, we have  $\bigcup_{x=1}^{j-1} C_{b-1}(x) \cup B(\sum_{x=1}^{j-1} |C_{b-1}(x)| + 1, b) \succ \bigcup_{x=1}^{j-2} C_{b-1}(x) \cup B(\sum_{x=1}^{j-2} |C_{b-1}(x)| + 1, b)$

Based on the two properties, a  $O(\log(n))$  search can be designed to solve (3.2), and thus a  $O(n \log(n))$  algorithm can be designed to solve (2.1).
